# Supplementary material for: VersaTune: An Efficient Data Composition Framework for Training Multi-Capability LLMs
Source: arXiv:2411.11266 source file (2025-05-19)
Supplement: Supplementary file 1 [file appendix_table_old.tex]

\begin{table*}[ht]
\vskip -0.2in
    \centering
    \caption{Ablation studies on multi-ability fostering, we compare the performances of \textbf{\ours} and fix domain weights based on the detected knowledge distribution (\textbf{\ours Constant}) across different models. The domain performance scores were calculated as the mean of respective domain benchmark scores. ``Avg'' denotes the average performance across all domain-specific tasks. ${\color{green} \uparrow}$ and ${\color{red} \downarrow}$ indicate an increase or decrease in scores comparing to the \textbf{\ours} strategy.}
    \label{tab:multi_ability_avg_ablation}
    \resizebox{0.8\textwidth}{!}{
        \begin{tabular}{ccccccccc}
            \toprule
                Model & Method & \multicolumn{1}{|c}{Law} & Medical & Finance & Science & Code & \multicolumn{1}{c|}{General} & Avg. \\
            \midrule
             \multirow{2}{*}{LLaMA-2-7B} & \ours Constant & \multicolumn{1}{|c}{28.51$^{\color{red} \downarrow }$} & 33.45$^{\color{red} \downarrow }$ & 21.09$^{\color{red} \downarrow }$ & 47.89$^{\color{red} \downarrow }$ & 13.47$^{\color{red} \downarrow }$ & 47.10$^{\color{red} \downarrow }$ & \multicolumn{1}{|c}{31.92$^{\color{red} \downarrow }$} \\
              & \ours & \multicolumn{1}{|c}{29.75} & 37.90 & 32.66& 53.41& 15.65& 48.22& \multicolumn{1}{|c}{36.27} \\
              \midrule
              \multirow{2}{*}{LLaMA-3-8B} & \ours Constant & \multicolumn{1}{|c}{42.80$^{\color{red} \downarrow }$} & 33.74$^{\color{red} \downarrow }$ & 31.60$^{\color{red} \downarrow }$ & 55.41$^{\color{red} \downarrow }$ & 31.55$^{\color{red} \downarrow }$ & 49.48$^{\color{red} \downarrow }$ & \multicolumn{1}{|c}{40.76$^{\color{red} \downarrow }$} \\
              & \ours & \multicolumn{1}{|c}{43.77} & 43.97& 41.19& 58.64& 32.28& 51.20& \multicolumn{1}{|c}{45.18} \\
              \midrule
              \multirow{2}{*}{Qwen-1.5-7B} & \ours Constant & \multicolumn{1}{|c}{36.75$^{\color{red} \downarrow }$} & 27.94$^{\color{red} \downarrow }$ & 46.29$^{\color{red} \downarrow }$ & 47.86$^{\color{red} \downarrow }$ & 34.04$^{\color{red} \downarrow }$ & 56.59$^{\color{red} \downarrow }$ & \multicolumn{1}{|c}{41.58$^{\color{red} \downarrow }$} \\
              & \ours & \multicolumn{1}{|c}{38.00} & 31.36& 56.08& 54.44& 36.15& 57.24& \multicolumn{1}{|c}{45.55} \\
              \midrule
              \multirow{2}{*}{Qwen-2-7B} & \ours Constant & \multicolumn{1}{|c}{39.29$^{\color{red} \downarrow }$} & 40.01$^{\color{red} \downarrow }$ & 50.73$^{\color{red} \downarrow }$ & 56.61$^{\color{red} \downarrow }$ & 51.29$^{\color{red} \downarrow }$ & 60.57$^{\color{red} \downarrow }$ & \multicolumn{1}{|c}{49.75$^{\color{red} \downarrow }$} \\
              & \ours & \multicolumn{1}{|c}{43.05} & 43.36& 64.67& 61.00& 52.90& 60.85& \multicolumn{1}{|c}{54.31} \\
              \midrule
             \multirow{2}{*}{Qwen-2.5-7B} & \ours Constant & \multicolumn{1}{|c}{41.99$^{\color{red} \downarrow }$} & 39.96$^{\color{red} \downarrow }$ & 55.71$^{\color{red} \downarrow }$ & 64.00$^{\color{red} \downarrow }$ & 55.63$^{\color{red} \downarrow }$ & 60.82$^{\color{red} \downarrow }$ & \multicolumn{1}{|c}{53.02$^{\color{red} \downarrow }$} \\
              & \ours & \multicolumn{1}{|c}{44.20} & 43.19& 65.79& 71.15& 60.97& 61.82& \multicolumn{1}{|c}{57.85} \\
              \midrule
              \multirow{2}{*}{LLaMA-2-13B} & \ours Constant & \multicolumn{1}{|c}{46.26$^{\color{red} \downarrow }$} & 41.72$^{\color{red} \downarrow }$ & 38.90$^{\color{red} \downarrow }$ & 56.12$^{\color{red} \downarrow }$ & 42.75$^{\color{red} \downarrow }$ & 56.09$^{\color{red} \downarrow }$ & \multicolumn{1}{|c}{46.97$^{\color{red} \downarrow }$} \\
              & \ours & \multicolumn{1}{|c}{48.01} & 46.73 & 47.30 & 63.36 & 46.15 & 57.14 & \multicolumn{1}{|c}{51.45} \\
              \midrule
              \multirow{2}{*}{Qwen-2.5-14B} & \ours Constant & \multicolumn{1}{|c}{51.29$^{\color{red} \downarrow }$} & 44.88$^{\color{red} \downarrow }$ & 34.14$^{\color{red} \downarrow }$ & 63.39$^{\color{red} \downarrow }$ & 78.53$^{\color{red} \downarrow }$ & 65.75$^{\color{red} \downarrow }$ & \multicolumn{1}{|c}{56.33$^{\color{red} \downarrow }$} \\
              & \ours & \multicolumn{1}{|c}{53.59} & 47.70 & 72.26 & 72.88 & 82.06 & 65.75 & \multicolumn{1}{|c}{65.71} \\
            \bottomrule
        \end{tabular}
    }
    \vskip -0.2in
\end{table*}

\begin{table*}[htbp]
\vskip -0.1in
    \centering
    \begin{minipage}{0.49\linewidth}
        \centering
        \caption{Results of law related tasks on multi-ability fostering.}
        \resizebox{0.807\linewidth}{!}{ % 1.017\linewidth
            \begin{tabular}{cccc}
                \toprule
                Model & Method & \multicolumn{1}{|c}{LegalBench} & LawBench \\
                \midrule
               \multirow{4}{*}{LLaMA-2-7B} & Uniform Distribution & \multicolumn{1}{|c}{15.71} & 30.72 \\
              &  Inverse Distribution & \multicolumn{1}{|c}{13.23$^{\color{red} \downarrow }$} & 26.94$^{\color{red} \downarrow }$ \\
              &  \ours Constant & \multicolumn{1}{|c}{\underline{21.47}$^{\color{green} \uparrow }$} & \underline{35.55}$^{\color{green} \uparrow }$ \\
              & \ours & \multicolumn{1}{|c}{\textbf{23.18}$^{\color{green} \uparrow }$} & \textbf{36.31}$^{\color{green} \uparrow }$ \\
              \midrule
               \multirow{4}{*}{LLaMA-3-8B} & Uniform Distribution & \multicolumn{1}{|c}{33.52} & 31.16 \\
              &  Inverse Distribution & \multicolumn{1}{|c}{27.83$^{\color{red} \downarrow }$} & 27.48$^{\color{red} \downarrow }$ \\
              &  \ours Constant & \multicolumn{1}{|c}{\underline{47.85}$^{\color{green} \uparrow }$} & \underline{37.75}$^{\color{green} \uparrow }$ \\
              & \ours & \multicolumn{1}{|c}{\textbf{49.67}$^{\color{green} \uparrow }$} & \textbf{37.87}$^{\color{green} \uparrow }$ \\
              \midrule
               \multirow{4}{*}{Qwen-1.5-7B} & Uniform Distribution & \multicolumn{1}{|c}{30.33} & 33.49 \\
              &  Inverse Distribution & \multicolumn{1}{|c}{29.80$^{\color{red} \downarrow }$} & 30.13$^{\color{red} \downarrow }$ \\
              &  \ours Constant & \multicolumn{1}{|c}{\underline{37.97}$^{\color{green} \uparrow }$} & \underline{35.52}$^{\color{green} \uparrow }$ \\
              & \ours & \multicolumn{1}{|c}{\textbf{40.04}$^{\color{green} \uparrow }$} & \textbf{35.95}$^{\color{green} \uparrow }$ \\
              \midrule
               \multirow{4}{*}{Qwen-2-7B} & Uniform Distribution & \multicolumn{1}{|c}{39.05} & 31.99 \\
              &  Inverse Distribution & \multicolumn{1}{|c}{34.01$^{\color{red} \downarrow }$} & 27.81$^{\color{red} \downarrow }$ \\
              &  \ours Constant & \multicolumn{1}{|c}{\underline{45.86}$^{\color{green} \uparrow }$} & \underline{32.72}$^{\color{green} \uparrow }$ \\
              & \ours & \multicolumn{1}{|c}{\textbf{50.56}$^{\color{green} \uparrow }$} & \textbf{35.54}$^{\color{green} \uparrow }$ \\
              \midrule
               \multirow{4}{*}{Qwen-2.5-7B} & Uniform Distribution & \multicolumn{1}{|c}{40.11} & 31.48 \\
              &  Inverse Distribution & \multicolumn{1}{|c}{36.36$^{\color{red} \downarrow }$} & 26.98$^{\color{red} \downarrow }$ \\
              &  \ours Constant & \multicolumn{1}{|c}{\underline{48.78}$^{\color{green} \uparrow }$} & \underline{35.20}$^{\color{green} \uparrow }$ \\
              & \ours & \multicolumn{1}{|c}{\textbf{51.65}$^{\color{green} \uparrow }$} & \textbf{36.75}$^{\color{green} \uparrow }$ \\
              \midrule
               \multirow{4}{*}{LLaMA-2-13B} & Uniform Distribution & \multicolumn{1}{|c}{47.66} & 34.85 \\
              &  Inverse Distribution & \multicolumn{1}{|c}{40.12$^{\color{red} \downarrow }$} & 30.67$^{\color{red} \downarrow }$ \\
              &  \ours Constant & \multicolumn{1}{|c}{\underline{53.79}$^{\color{green} \uparrow }$} & \underline{38.73}$^{\color{green} \uparrow }$ \\
              & \ours & \multicolumn{1}{|c}{\textbf{55.87}$^{\color{green} \uparrow }$} & \textbf{40.14}$^{\color{green} \uparrow }$ \\
              \midrule
               \multirow{4}{*}{Qwen-2.5-14B} & Uniform Distribution & \multicolumn{1}{|c}{50.73} & 39.49 \\
              &  Inverse Distribution & \multicolumn{1}{|c}{46.08$^{\color{red} \downarrow }$} & 35.36$^{\color{red} \downarrow }$ \\
              &  \ours Constant & \multicolumn{1}{|c}{\underline{56.94}$^{\color{green} \uparrow }$} & \underline{45.64}$^{\color{green} \uparrow }$ \\
              & \ours & \multicolumn{1}{|c}{\textbf{60.59}$^{\color{green} \uparrow }$} & \textbf{46.58}$^{\color{green} \uparrow }$ \\
                \bottomrule
            \end{tabular}
        }
        \label{tab:multi_ability_law}
    \end{minipage}%
    \hfill
    \begin{minipage}{0.49\linewidth}
        \centering
        \caption{Results of medical tasks on multi-ability fostering.}
        \resizebox{0.77\linewidth}{!}{ % 0.98\linewidth
            \begin{tabular}{cccc}
                \toprule
                Model & Method & \multicolumn{1}{|c}{MedQA} & MedMCQA \\
                \midrule
               \multirow{4}{*}{LLaMA-2-7B} & Uniform Distribution & \multicolumn{1}{|c}{23.45} & 27.57 \\
              &  Inverse Distribution & \multicolumn{1}{|c}{21.38$^{\color{red} \downarrow }$} & 26.52$^{\color{red} \downarrow }$ \\
              &  \ours Constant & \multicolumn{1}{|c}{\underline{30.17}$^{\color{green} \uparrow }$} & \underline{36.72}$^{\color{green} \uparrow }$ \\
              & \ours & \multicolumn{1}{|c}{\textbf{35.04}$^{\color{green} \uparrow }$} & \textbf{40.75}$^{\color{green} \uparrow }$ \\
              \midrule
               \multirow{4}{*}{LLaMA-3-8B} & Uniform Distribution & \multicolumn{1}{|c}{31.03} & 10.26 \\
              &  Inverse Distribution & \multicolumn{1}{|c}{25.51$^{\color{red} \downarrow }$} & 8.77$^{\color{red} \downarrow }$ \\
              &  \ours Constant & \multicolumn{1}{|c}{\underline{37.33}$^{\color{green} \uparrow }$} & \underline{30.15}$^{\color{green} \uparrow }$ \\
              & \ours & \multicolumn{1}{|c}{\textbf{42.21}$^{\color{green} \uparrow }$} & \textbf{45.72}$^{\color{green} \uparrow }$ \\
              \midrule
               \multirow{4}{*}{Qwen-1.5-7B} & Uniform Distribution & \multicolumn{1}{|c}{21.27} & 12.14 \\
              &  Inverse Distribution & \multicolumn{1}{|c}{16.15$^{\color{red} \downarrow }$} & 9.91$^{\color{red} \downarrow }$ \\
              &  \ours Constant & \multicolumn{1}{|c}{\underline{25.60}$^{\color{green} \uparrow }$} & \underline{30.28}$^{\color{green} \uparrow }$ \\
              & \ours & \multicolumn{1}{|c}{\textbf{30.47}$^{\color{green} \uparrow }$} & \textbf{32.24}$^{\color{green} \uparrow }$ \\
              \midrule
               \multirow{4}{*}{Qwen-2-7B} & Uniform Distribution & \multicolumn{1}{|c}{35.07} & 17.73 \\
              &  Inverse Distribution & \multicolumn{1}{|c}{23.90$^{\color{red} \downarrow }$} & 16.31$^{\color{red} \downarrow }$ \\
              &  \ours Constant & \multicolumn{1}{|c}{\underline{40.89}$^{\color{green} \uparrow }$} & \underline{39.13}$^{\color{green} \uparrow }$ \\
              & \ours & \multicolumn{1}{|c}{\textbf{45.48}$^{\color{green} \uparrow }$} & \textbf{41.24}$^{\color{green} \uparrow }$ \\
              \midrule
              \multirow{4}{*}{Qwen-2.5-7B} & Uniform Distribution & \multicolumn{1}{|c}{25.17} & 25.84 \\
              &  Inverse Distribution & \multicolumn{1}{|c}{24.16$^{\color{red} \downarrow }$} & 19.35$^{\color{red} \downarrow }$ \\
              &  \ours Constant & \multicolumn{1}{|c}{\underline{30.20}$^{\color{green} \uparrow }$} & \underline{49.71}$^{\color{green} \uparrow }$ \\
              & \ours & \multicolumn{1}{|c}{\textbf{34.28}$^{\color{green} \uparrow }$} & \textbf{52.09}$^{\color{green} \uparrow }$ \\
              \midrule
               \multirow{4}{*}{LLaMA-2-13B} & Uniform Distribution & \multicolumn{1}{|c}{32.98} & 36.54 \\
              &  Inverse Distribution & \multicolumn{1}{|c}{26.27$^{\color{red} \downarrow }$} & 28.78$^{\color{red} \downarrow }$ \\
              &  \ours Constant & \multicolumn{1}{|c}{\underline{40.69}$^{\color{green} \uparrow }$} & \underline{42.74}$^{\color{green} \uparrow }$ \\
              & \ours & \multicolumn{1}{|c}{\textbf{45.78}$^{\color{green} \uparrow }$} & \textbf{47.67}$^{\color{green} \uparrow }$ \\
              \midrule
               \multirow{4}{*}{Qwen-2.5-14B} & Uniform Distribution & \multicolumn{1}{|c}{47.85} & 38.71 \\
              &  Inverse Distribution & \multicolumn{1}{|c}{45.75$^{\color{red} \downarrow }$} & 32.56$^{\color{red} \downarrow }$ \\
              &  \ours Constant & \multicolumn{1}{|c}{\underline{48.11}$^{\color{green} \uparrow }$} & \underline{41.64}$^{\color{green} \uparrow }$ \\
              & \ours & \multicolumn{1}{|c}{\textbf{50.24}$^{\color{green} \uparrow }$} & \textbf{45.15}$^{\color{green} \uparrow }$ \\
                \bottomrule
            \end{tabular}
        }
        \label{tab:multi_ability_results_medical}
    \end{minipage}
\end{table*}

\begin{table}[ht] % htbp
    \centering
    \begin{minipage}{0.49\linewidth}
        \centering
        \caption{Results of finance related tasks on multi-ability fostering.}
        \resizebox{0.883\linewidth}{!}{ % 0.983\linewidth
            \begin{tabular}{cccc}
                \toprule
                Model & Method & \multicolumn{1}{|c}{FinEval} & FinanceIQ \\
                \midrule
               \multirow{4}{*}{LLaMA-2-7B} & Uniform Distribution & \multicolumn{1}{|c}{33.50} & 2.71 \\
              &  Inverse Distribution & \multicolumn{1}{|c}{32.96$^{\color{red} \downarrow }$} & 2.53$^{\color{red} \downarrow }$ \\
              &  \ours Constant & \multicolumn{1}{|c}{\underline{35.89}$^{\color{green} \uparrow }$} & \underline{6.28}$^{\color{green} \uparrow }$ \\
              & \ours & \multicolumn{1}{|c}{\textbf{36.27}$^{\color{green} \uparrow }$} & \textbf{29.04}$^{\color{green} \uparrow }$ \\
              \midrule
               \multirow{4}{*}{LLaMA-3-8B} & Uniform Distribution & \multicolumn{1}{|c}{34.83} & 4.97 \\
              &  Inverse Distribution & \multicolumn{1}{|c}{33.71$^{\color{red} \downarrow }$} & 3.31$^{\color{red} \downarrow }$ \\
               &  \ours Constant & \multicolumn{1}{|c}{\underline{37.93}$^{\color{green} \uparrow }$} & \underline{25.27}$^{\color{green} \uparrow }$ \\
              & \ours & \multicolumn{1}{|c}{\textbf{38.80}$^{\color{green} \uparrow }$} & \textbf{43.58}$^{\color{green} \uparrow }$ \\
              \midrule
               \multirow{4}{*}{Qwen-1.5-7B} & Uniform Distribution & \multicolumn{1}{|c}{53.87} & 14.17 \\
              &  Inverse Distribution & \multicolumn{1}{|c}{53.80$^{\color{red} \downarrow }$} & 12.44$^{\color{red} \downarrow }$ \\
              &  \ours Constant & \multicolumn{1}{|c}{\underline{55.06}$^{\color{green} \uparrow }$} & \underline{37.52}$^{\color{green} \uparrow }$ \\
              & \ours & \multicolumn{1}{|c}{\textbf{55.52}$^{\color{green} \uparrow }$} & \textbf{56.63}$^{\color{green} \uparrow }$ \\
              \midrule
               \multirow{4}{*}{Qwen-2-7B} & Uniform Distribution & \multicolumn{1}{|c}{59.49} & 14.62 \\
              &  Inverse Distribution & \multicolumn{1}{|c}{56.53$^{\color{red} \downarrow }$} & 11.30$^{\color{red} \downarrow }$ \\
              &  \ours Constant & \multicolumn{1}{|c}{\underline{60.63}$^{\color{green} \uparrow }$} & \underline{40.82}$^{\color{green} \uparrow }$ \\
              & \ours & \multicolumn{1}{|c}{\textbf{60.95}$^{\color{green} \uparrow }$} & \textbf{68.39}$^{\color{green} \uparrow }$ \\
              \midrule
               \multirow{4}{*}{Qwen-2.5-7B} & Uniform Distribution & \multicolumn{1}{|c}{59.58} & 31.66 \\
              &  Inverse Distribution & \multicolumn{1}{|c}{57.07$^{\color{red} \downarrow }$} & 29.25$^{\color{red} \downarrow }$ \\
              &  \ours Constant & \multicolumn{1}{|c}{\textbf{62.94}$^{\color{green} \uparrow }$} & \underline{48.47}$^{\color{green} \uparrow }$ \\
              & \ours & \multicolumn{1}{|c}{\underline{62.48}$^{\color{green} \uparrow }$} & \textbf{69.09}$^{\color{green} \uparrow }$ \\
              \midrule
               \multirow{4}{*}{LLaMA-2-13B} & Uniform Distribution & \multicolumn{1}{|c}{37.54} & 32.85 \\
              &  Inverse Distribution & \multicolumn{1}{|c}{36.67$^{\color{red} \downarrow }$} & 26.76$^{\color{red} \downarrow }$ \\
              &  \ours Constant & \multicolumn{1}{|c}{\underline{39.33}$^{\color{green} \uparrow }$} & \underline{38.47}$^{\color{green} \uparrow }$ \\
              & \ours & \multicolumn{1}{|c}{\textbf{39.48}$^{\color{green} \uparrow }$} & \textbf{55.12}$^{\color{green} \uparrow }$ \\
              \midrule
               \multirow{4}{*}{Qwen-2.5-14B} & Uniform Distribution & \multicolumn{1}{|c}{64.72} & 64.39 \\
              &  Inverse Distribution & \multicolumn{1}{|c}{64.88$^{\color{green} \uparrow }$} & 60.53$^{\color{red} \downarrow }$ \\
              &  \ours Constant & \multicolumn{1}{|c}{\underline{65.03}$^{\color{green} \uparrow }$} & \underline{73.24}$^{\color{green} \uparrow }$ \\
              & \ours & \multicolumn{1}{|c}{\textbf{65.84}$^{\color{green} \uparrow }$} & \textbf{78.68}$^{\color{green} \uparrow }$ \\
                \bottomrule
            \end{tabular}
        }
        \label{tab:multi_ability_results_finance}
    \end{minipage}%
    \hfill
    \begin{minipage}{0.49\linewidth}
        \centering
        \caption{Results of science related tasks on multi-ability fostering.}
        \resizebox{0.9\linewidth}{!}{ % \linewidth
            \begin{tabular}{cccc}
                \toprule
                Model & Method & \multicolumn{1}{|c}{SciEval} & MMLU-Sci \\
                \midrule
               \multirow{4}{*}{LLaMA-2-7B} & Uniform Distribution & \multicolumn{1}{|c}{9.30} & 42.89 \\
              &  Inverse Distribution & \multicolumn{1}{|c}{8.98$^{\color{red} \downarrow }$} & 39.67$^{\color{red} \downarrow }$ \\
              &  \ours Constant & \multicolumn{1}{|c}{\underline{49.91}$^{\color{green} \uparrow }$} & \underline{45.87}$^{\color{green} \uparrow }$ \\
              & \ours & \multicolumn{1}{|c}{\textbf{56.75}$^{\color{green} \uparrow }$} & \textbf{50.06}$^{\color{green} \uparrow }$ \\
              \midrule
               \multirow{4}{*}{LLaMA-3-8B} & Uniform Distribution & \multicolumn{1}{|c}{6.51} & 50.17 \\
              &  Inverse Distribution & \multicolumn{1}{|c}{6.09$^{\color{red} \downarrow }$} & 46.62$^{\color{red} \downarrow }$ \\
              &  \ours Constant & \multicolumn{1}{|c}{\underline{54.77}$^{\color{green} \uparrow }$} & \underline{56.04}$^{\color{green} \uparrow }$ \\
              & \ours & \multicolumn{1}{|c}{\textbf{56.67}$^{\color{green} \uparrow }$} & \textbf{60.61}$^{\color{green} \uparrow }$ \\
              \midrule
               \multirow{4}{*}{Qwen-1.5-7B} & Uniform Distribution & \multicolumn{1}{|c}{7.63} & 50.67 \\
              &  Inverse Distribution & \multicolumn{1}{|c}{6.54$^{\color{red} \downarrow }$} & 48.52$^{\color{red} \downarrow }$ \\
              &  \ours Constant & \multicolumn{1}{|c}{\underline{38.39}$^{\color{green} \uparrow }$} & \underline{57.33}$^{\color{green} \uparrow }$ \\
              & \ours & \multicolumn{1}{|c}{\textbf{47.76}$^{\color{green} \uparrow }$} & \textbf{61.11}$^{\color{green} \uparrow }$ \\
              \midrule
               \multirow{4}{*}{Qwen-2-7B} & Uniform Distribution & \multicolumn{1}{|c}{25.30} & 62.73 \\
              &  Inverse Distribution & \multicolumn{1}{|c}{18.57$^{\color{red} \downarrow }$} & 58.25$^{\color{red} \downarrow }$ \\
              &  \ours Constant & \multicolumn{1}{|c}{\underline{45.93}$^{\color{green} \uparrow }$} & \underline{67.29}$^{\color{green} \uparrow }$ \\
              & \ours & \multicolumn{1}{|c}{\textbf{51.58}$^{\color{green} \uparrow }$} & \textbf{70.42}$^{\color{green} \uparrow }$ \\
              \midrule
               \multirow{4}{*}{Qwen-2.5-7B} & Uniform Distribution & \multicolumn{1}{|c}{19.88} & 65.84 \\
              &  Inverse Distribution & \multicolumn{1}{|c}{16.68$^{\color{red} \downarrow }$} & 62.78$^{\color{red} \downarrow }$ \\
              &  \ours Constant & \multicolumn{1}{|c}{\underline{56.04}$^{\color{green} \uparrow }$} & \underline{71.96}$^{\color{green} \uparrow }$ \\
              & \ours & \multicolumn{1}{|c}{\textbf{68.14}$^{\color{green} \uparrow }$} & \textbf{74.16}$^{\color{green} \uparrow }$ \\
              \midrule
               \multirow{4}{*}{LLaMA-2-13B} & Uniform Distribution & \multicolumn{1}{|c}{45.72} & 50.77 \\
              &  Inverse Distribution & \multicolumn{1}{|c}{38.96$^{\color{red} \downarrow }$} & 48.68$^{\color{red} \downarrow }$ \\
              &  \ours Constant & \multicolumn{1}{|c}{\underline{57.13}$^{\color{green} \uparrow }$} & \underline{55.10}$^{\color{green} \uparrow }$ \\
              & \ours & \multicolumn{1}{|c}{\textbf{63.87}$^{\color{green} \uparrow }$} & \textbf{62.84}$^{\color{green} \uparrow }$ \\
              \midrule
               \multirow{4}{*}{Qwen-2.5-14B} & Uniform Distribution & \multicolumn{1}{|c}{39.74} & 73.45 \\
              &  Inverse Distribution & \multicolumn{1}{|c}{27.68$^{\color{red} \downarrow }$} & 68.22$^{\color{red} \downarrow }$ \\
              &  \ours Constant & \multicolumn{1}{|c}{\underline{48.31}$^{\color{green} \uparrow }$} & \underline{78.46}$^{\color{green} \uparrow }$ \\
              & \ours & \multicolumn{1}{|c}{\textbf{62.89}$^{\color{green} \uparrow }$} & \textbf{82.86}$^{\color{green} \uparrow }$ \\
                \bottomrule
            \end{tabular}
        }
        \label{tab:multi_ability_results_science}
    \end{minipage}
    \vskip -0.2in
\end{table}


\begin{table}[ht]
\vskip -0.1in
    \centering
    \begin{minipage}{0.49\linewidth}
        \centering
        \caption{Results of code related tasks on multi-ability fostering.}
        \resizebox{0.89\linewidth}{!}{ % 0.99\linewidth
            \begin{tabular}{cccc}
                \toprule
                Model & Method & \multicolumn{1}{|c}{HumanEval} & MBPP \\ % BigCodeBench
                \midrule
               \multirow{4}{*}{LLaMA-2-7B} & Uniform Distribution & \multicolumn{1}{|c}{5.67} & 3.44 \\
              &  Inverse Distribution & \multicolumn{1}{|c}{3.47$^{\color{red} \downarrow }$} & 2.42$^{\color{red} \downarrow }$ \\
              &  \ours Constant & \multicolumn{1}{|c}{\underline{12.47}$^{\color{green} \uparrow }$} & \underline{14.47}$^{\color{green} \uparrow }$ \\
              & \ours & \multicolumn{1}{|c}{\textbf{15.62}$^{\color{green} \uparrow }$} & \textbf{15.68}$^{\color{green} \uparrow }$ \\
              \midrule
               \multirow{4}{*}{LLaMA-3-8B} & Uniform Distribution & \multicolumn{1}{|c}{22.94} & 28.85 \\
              &  Inverse Distribution & \multicolumn{1}{|c}{19.67$^{\color{red} \downarrow }$} & 24.34$^{\color{red} \downarrow }$ \\
              &  \ours Constant & \multicolumn{1}{|c}{\textbf{29.88}$^{\color{green} \uparrow }$} & \underline{33.22}$^{\color{green} \uparrow }$ \\
              & \ours & \multicolumn{1}{|c}{\underline{28.91}$^{\color{green} \uparrow }$} & \textbf{35.65}$^{\color{green} \uparrow }$ \\
              \midrule
               \multirow{4}{*}{Qwen-1.5-7B} & Uniform Distribution & \multicolumn{1}{|c}{32.86} & 25.86 \\
              &  Inverse Distribution & \multicolumn{1}{|c}{28.55$^{\color{red} \downarrow }$} & 23.94$^{\color{red} \downarrow }$ \\
              &  \ours Constant & \multicolumn{1}{|c}{\underline{38.41}$^{\color{green} \uparrow }$} & \underline{29.67}$^{\color{green} \uparrow }$ \\
              & \ours & \multicolumn{1}{|c}{\textbf{40.49}$^{\color{green} \uparrow }$} & \textbf{31.80}$^{\color{green} \uparrow }$ \\
              \midrule
               \multirow{4}{*}{Qwen-2-7B} & Uniform Distribution & \multicolumn{1}{|c}{53.26} & 37.82 \\
              &  Inverse Distribution & \multicolumn{1}{|c}{50.65$^{\color{red} \downarrow }$} & 33.63$^{\color{red} \downarrow }$ \\
              &  \ours Constant & \multicolumn{1}{|c}{\underline{56.71}$^{\color{green} \uparrow }$} & \underline{45.87}$^{\color{green} \uparrow }$ \\
              & \ours & \multicolumn{1}{|c}{\textbf{58.15}$^{\color{green} \uparrow }$} & \textbf{47.64}$^{\color{green} \uparrow }$ \\
              \midrule
               \multirow{4}{*}{Qwen-2.5-7B} & Uniform Distribution & \multicolumn{1}{|c}{55.64} & 46.86 \\
              &  Inverse Distribution & \multicolumn{1}{|c}{52.97$^{\color{red} \downarrow }$} & 44.63$^{\color{red} \downarrow }$ \\
              &  \ours Constant & \multicolumn{1}{|c}{\underline{59.15}$^{\color{green} \uparrow }$} & \underline{52.10}$^{\color{green} \uparrow }$ \\
              & \ours & \multicolumn{1}{|c}{\textbf{60.68}$^{\color{green} \uparrow }$} & \textbf{61.25}$^{\color{green} \uparrow }$ \\
              \midrule
               \multirow{4}{*}{LLaMA-2-13B} & Uniform Distribution & \multicolumn{1}{|c}{36.54} & 38.55 \\
              &  Inverse Distribution & \multicolumn{1}{|c}{28.78$^{\color{red} \downarrow }$} & 35.83$^{\color{red} \downarrow }$ \\
              &  \ours Constant & \multicolumn{1}{|c}{\underline{42.74}$^{\color{green} \uparrow }$} & \underline{42.76}$^{\color{green} \uparrow }$ \\
              & \ours & \multicolumn{1}{|c}{\textbf{47.67}$^{\color{green} \uparrow }$} & \textbf{44.62}$^{\color{green} \uparrow }$ \\
              \midrule
               \multirow{4}{*}{Qwen-2.5-14B} & Uniform Distribution & \multicolumn{1}{|c}{68.75} & 72.14 \\
              &  Inverse Distribution & \multicolumn{1}{|c}{63.36$^{\color{red} \downarrow }$} & 68.49$^{\color{red} \downarrow }$ \\
              &  \ours Constant & \multicolumn{1}{|c}{\underline{78.72}$^{\color{green} \uparrow }$} & \underline{78.33}$^{\color{green} \uparrow }$ \\
              & \ours & \multicolumn{1}{|c}{\textbf{82.64}$^{\color{green} \uparrow }$} & \textbf{81.48}$^{\color{green} \uparrow }$ \\
                \bottomrule
        \end{tabular}
        }
        \label{tab:multi_ability_results_code}
    \end{minipage}%
    \hfill
    \begin{minipage}{0.49\linewidth}
        \centering
        \caption{Results of general tasks on multi-ability fostering.}
        \resizebox{0.9\linewidth}{!}{ % 1\linewidth
            \begin{tabular}{cccc}
                \toprule
                Model & Method & \multicolumn{1}{|c}{AGIEval} & HellaSwag \\
                \midrule
               \multirow{4}{*}{LLaMA-2-7B} & Uniform Distribution & \multicolumn{1}{|c}{20.16} & 71.40 \\
              &  Inverse Distribution & \multicolumn{1}{|c}{18.83$^{\color{red} \downarrow }$} & 71.33$^{\color{red} \downarrow }$ \\
              &  \ours Constant & \multicolumn{1}{|c}{\underline{22.31}$^{\color{green} \uparrow }$} & \textbf{71.89}$^{\color{green} \uparrow }$ \\
              & \ours & \multicolumn{1}{|c}{\textbf{24.67}$^{\color{green} \uparrow }$} & \underline{71.76}$^{\color{green} \uparrow }$ \\
              \midrule
               \multirow{4}{*}{LLaMA-3-8B} & Uniform Distribution & \multicolumn{1}{|c}{23.87} & 73.26 \\
              &  Inverse Distribution & \multicolumn{1}{|c}{23.45$^{\color{red} \downarrow }$} & 72.40$^{\color{red} \downarrow }$ \\
               &  \ours Constant & \multicolumn{1}{|c}{\underline{25.62}$^{\color{green} \uparrow }$} & \underline{73.33}$^{\color{green} \uparrow }$ \\
              & \ours & \multicolumn{1}{|c}{\textbf{28.78}$^{\color{green} \uparrow }$} & \textbf{73.62}$^{\color{green} \uparrow }$ \\
              \midrule
               \multirow{4}{*}{Qwen-1.5-7B} & Uniform Distribution & \multicolumn{1}{|c}{39.19} & 69.80 \\
              &  Inverse Distribution & \multicolumn{1}{|c}{39.56$^{\color{green} \uparrow }$} & 69.59$^{\color{red} \downarrow }$ \\
               &  \ours Constant & \multicolumn{1}{|c}{\underline{42.50}$^{\color{green} \uparrow }$} & \underline{70.67}$^{\color{green} \uparrow }$ \\
              & \ours & \multicolumn{1}{|c}{\textbf{42.96}$^{\color{green} \uparrow }$} & \textbf{71.51}$^{\color{green} \uparrow }$ \\
              \midrule
               \multirow{4}{*}{Qwen-2-7B} & Uniform Distribution & \multicolumn{1}{|c}{47.31} & \underline{73.60} \\
              &  Inverse Distribution & \multicolumn{1}{|c}{45.74$^{\color{red} \downarrow }$} & 73.52$^{\color{red} \downarrow }$ \\
               &  \ours Constant & \multicolumn{1}{|c}{\textbf{48.16}$^{\color{green} \uparrow }$} & 72.98$^{\color{red} \downarrow }$ \\
              & \ours & \multicolumn{1}{|c}{\underline{48.02}$^{\color{green} \uparrow }$} & \textbf{73.67}$^{\color{green} \uparrow }$ \\
              \midrule
               \multirow{4}{*}{Qwen-2.5-7B} & Uniform Distribution & \multicolumn{1}{|c}{45.42} & 73.69 \\
              &  Inverse Distribution & \multicolumn{1}{|c}{45.67$^{\color{green} \uparrow }$} & 72.92$^{\color{red} \downarrow }$ \\
               &  \ours Constant & \multicolumn{1}{|c}{\underline{47.75}$^{\color{green} \uparrow }$} & \underline{73.88}$^{\color{green} \uparrow }$ \\
              & \ours & \multicolumn{1}{|c}{\textbf{49.73}$^{\color{green} \uparrow }$} & \textbf{73.90}$^{\color{green} \uparrow }$ \\
              \midrule
               \multirow{4}{*}{LLaMA-2-13B} & Uniform Distribution & \multicolumn{1}{|c}{36.89} & 73.50 \\
              &  Inverse Distribution & \multicolumn{1}{|c}{36.67$^{\color{red} \downarrow }$} & 73.11$^{\color{red} \downarrow }$ \\
               &  \ours Constant & \multicolumn{1}{|c}{\underline{37.91}$^{\color{green} \uparrow }$} & \underline{74.27}$^{\color{green} \uparrow }$ \\
              & \ours & \multicolumn{1}{|c}{\textbf{39.64}$^{\color{green} \uparrow }$} & \textbf{74.63}$^{\color{green} \uparrow }$ \\
              \midrule
               \multirow{4}{*}{Qwen-2.5-14B} & Uniform Distribution & \multicolumn{1}{|c}{54.92} & 75.88 \\
              &  Inverse Distribution & \multicolumn{1}{|c}{54.87$^{\color{red} \downarrow }$} & 75.42$^{\color{red} \downarrow }$ \\
               &  \ours Constant & \multicolumn{1}{|c}{\underline{55.04}$^{\color{green} \uparrow }$} & \textbf{76.45}$^{\color{green} \uparrow }$ \\
              & \ours & \multicolumn{1}{|c}{\textbf{55.52}$^{\color{green} \uparrow }$} & \underline{75.98}$^{\color{green} \uparrow }$ \\
                \bottomrule
            \end{tabular}
        }
        \label{tab:multi_ability_results_general}
    \end{minipage}
\end{table}
